# Supplementary material for: Multiple imputation for multilevel data with continuous and binary variables
Source: arXiv:1702.00971 ancillary file (2017-11-27)
Supplement: Supplementary file 1 [file Tables_supp_review.pdf]

# 1 Supplementary files

The following tables provide inference results for configurations which are not discussed in the main text. Point estimate, relative bias, model standard error, empirical standard error, 95% coverage and RMSE for analysis model's parameters and for several methods (Full data, JM-jomo, FCS-GLM, FCS-2stage with REML estimator, FCS-2stage with moment estimator) are reported. Criteria are based on 500 incomplete datasets. Average time to multiply impute one dataset is indicated in minutes. Criteria related to the continuous (resp. binary) covariate are in light (resp. dark) grey. True values of the parameters are reported on the top of each table.

Table 11: Config 2: more sporadically missing values. True values are  $\beta_1 = -0.11$ ,  $\beta_2 = 0.03$ ,  $\sqrt{\psi_{00}} = 0.09$ ,  $\sqrt{\psi_{11}} = 0.02$ .

|                           | Full    | JM-jomo | FCS-GLM | FCS-2stageREML | FCS-2stageMM |
|---------------------------|---------|---------|---------|----------------|--------------|
| $\beta^{(1)}$ est         | -0.1101 | -0.1091 | -0.1100 | -0.1089        | -0.1089      |
| $\beta^{(1)}$ rbias (%)   | 0.1     | -0.8    | -0.0    | -1.0           | -1.0         |
| $\beta^{(1)}$ model se    | 0.0047  | 0.0059  | 0.0046  | 0.0055         | 0.0056       |
| $\beta^{(1)}$ emp se      | 0.0048  | 0.0055  | 0.0055  | 0.0055         | 0.0056       |
| $\beta^{(1)}$ 95% cover   | 93.8    | 95.2    | 88.5    | 94.2           | 93.2         |
| $\beta^{(1)}$ rmse        | 0.0048  | 0.0056  | 0.0055  | 0.0056         | 0.0057       |
| $\beta^{(2)}$ est         | 0.0301  | 0.0302  | 0.0299  | 0.0297         | 0.0300       |
| $\beta^{(2)}$ rbias (%)   | 0.2     | 0.5     | -0.3    | -0.9           | -0.1         |
| $\beta^{(2)}$ model se    | 0.0029  | 0.0051  | 0.0044  | 0.0047         | 0.0045       |
| $\beta^{(2)}$ emp se      | 0.0030  | 0.0045  | 0.0043  | 0.0042         | 0.0042       |
| $\beta^{(2)}$ 95% cover   | 94.2    | 95.0    | 94.2    | 95.5           | 95.9         |
| $\beta^{(2)}$ rmse        | 0.0030  | 0.0045  | 0.0043  | 0.0043         | 0.0042       |
| $\sqrt{\psi_0}$ est       | 0.0859  | 0.0907  | 0.0765  | 0.0860         | 0.0860       |
| $\sqrt{\psi_0}$ rbias (%) | -2.1    | 3.4     | -12.8   | -2.0           | -2.0         |
| $\sqrt{\psi_0}$ rmse      | 0.0154  | 0.0144  | 0.0181  | 0.0149         | 0.0149       |
| $\sqrt{\psi_1}$ est       | 0.0193  | 0.0215  | 0.0150  | 0.0197         | 0.0197       |
| $\sqrt{\psi_1}$ rbias (%) | -3.7    | 7.4     | -25.0   | -1.5           | -1.6         |
| $\sqrt{\psi_1}$ rmse      | 0.0041  | 0.0041  | 0.0065  | 0.0044         | 0.0044       |
| time                      |         | 7.7     | 105.8   | 2.3            | 0.9          |

Table 12: Config 3: more systematically missing values. True values are  $\beta_1 = -0.11$ ,  $\beta_2 = 0.03$ ,  $\sqrt{\psi_{00}} = 0.09$ ,  $\sqrt{\psi_{11}} = 0.02$ .

|                           | Full    | JM-jomo | FCS-GLM | FCS-2stageREML | FCS-2stageMM |
|---------------------------|---------|---------|---------|----------------|--------------|
| $\beta^{(1)}$ est         | -0.1101 | -0.1073 | -0.1098 | -0.1086        | -0.1087      |
| $\beta^{(1)}$ rbias (%)   | 0.1     | -2.4    | -0.2    | -1.3           | -1.2         |
| $\beta^{(1)}$ model se    | 0.0047  | 0.0079  | 0.0049  | 0.0064         | 0.0062       |
| $\beta^{(1)}$ emp se      | 0.0048  | 0.0059  | 0.0059  | 0.0061         | 0.0061       |
| $\beta^{(1)}$ 95% cover   | 93.8    | 98.0    | 88.6    | 94.4           | 94.6         |
| $\beta^{(1)}$ rmse        | 0.0048  | 0.0065  | 0.0059  | 0.0063         | 0.0063       |
| $\beta^{(2)}$ est         | 0.0301  | 0.0298  | 0.0301  | 0.0298         | 0.0301       |
| $\beta^{(2)}$ rbias (%)   | 0.2     | -0.8    | 0.3     | -0.8           | 0.5          |
| $\beta^{(2)}$ model se    | 0.0029  | 0.0085  | 0.0048  | 0.0065         | 0.0059       |
| $\beta^{(2)}$ emp se      | 0.0030  | 0.0055  | 0.0046  | 0.0048         | 0.0050       |
| $\beta^{(2)}$ 95% cover   | 94.2    | 98.2    | 95.7    | 98.2           | 95.2         |
| $\beta^{(2)}$ rmse        | 0.0030  | 0.0055  | 0.0046  | 0.0048         | 0.0050       |
| $\sqrt{\psi_0}$ est       | 0.0859  | 0.0982  | 0.0797  | 0.0871         | 0.0862       |
| $\sqrt{\psi_0}$ rbias (%) | -2.1    | 11.9    | -9.2    | -0.7           | -1.8         |
| $\sqrt{\psi_0}$ rmse      | 0.0154  | 0.0166  | 0.0164  | 0.0142         | 0.0145       |
| $\sqrt{\psi_1}$ est       | 0.0193  | 0.0235  | 0.0151  | 0.0195         | 0.0190       |
| $\sqrt{\psi_1}$ rbias (%) | -3.7    | 17.7    | -24.3   | -2.5           | -4.8         |
| $\sqrt{\psi_1}$ rmse      | 0.0041  | 0.0048  | 0.0066  | 0.0045         | 0.0048       |
| time                      |         | 7.7     | 102.7   | 1.9            | 0.8          |

Table 13: Config 5: Binary outcome. True values are  $\beta_1 = -1.44$ ,  $\beta_2 = 0.39$ ,  $\sqrt{\psi_{00}} = 1.24$ ,  $\sqrt{\psi_{11}} = 0.223606797749979$ .

|                           | Full    | JM-jomo | FCS-GLM | FCS-2stageREML | FCS-2stageMM |
|---------------------------|---------|---------|---------|----------------|--------------|
| $\beta^{(1)}$ est         | -1.4427 | -1.4312 | -1.4348 | -1.4306        | -1.4294      |
| $\beta^{(1)}$ rbias (%)   | 0.2     | -0.6    | -0.4    | -0.6           | -0.7         |
| $\beta^{(1)}$ model se    | 0.0607  | 0.1021  | 0.0722  | 0.1021         | 0.0981       |
| $\beta^{(1)}$ emp se      | 0.0638  | 0.0812  | 0.0794  | 0.0809         | 0.0830       |
| $\beta^{(1)}$ 95% cover   | 93.8    | 97.8    | 91.8    | 98.0           | 96.8         |
| $\beta^{(1)}$ rmse        | 0.0638  | 0.0817  | 0.0796  | 0.0815         | 0.0836       |
| $\beta^{(2)}$ est         | 0.3866  | 0.3843  | 0.3814  | 0.3791         | 0.3832       |
| $\beta^{(2)}$ rbias (%)   | -0.9    | -1.5    | -2.2    | -2.8           | -1.8         |
| $\beta^{(2)}$ model se    | 0.0440  | 0.0955  | 0.0703  | 0.0879         | 0.0754       |
| $\beta^{(2)}$ emp se      | 0.0446  | 0.0743  | 0.0684  | 0.0703         | 0.0685       |
| $\beta^{(2)}$ 95% cover   | 93.4    | 96.8    | 95.0    | 97.4           | 96.0         |
| $\beta^{(2)}$ rmse        | 0.0448  | 0.0745  | 0.0689  | 0.0711         | 0.0688       |
| $\sqrt{\psi_0}$ est       | 1.1934  | 1.2832  | 1.0848  | 1.3031         | 1.2793       |
| $\sqrt{\psi_0}$ rbias (%) | -3.8    | 3.4     | -12.6   | 5.0            | 3.1          |
| $\sqrt{\psi_0}$ rmse      | 0.2297  | 0.2190  | 0.2694  | 0.2558         | 0.2470       |
| $\sqrt{\psi_1}$ est       | 0.2025  | 0.2825  | 0.1584  | 0.2819         | 0.2700       |
| $\sqrt{\psi_1}$ rbias (%) | -9.4    | 26.4    | -29.2   | 26.1           | 20.8         |
| $\sqrt{\psi_1}$ rmse      | 0.0654  | 0.0821  | 0.0936  | 0.1027         | 0.0923       |
| time                      |         | 9.8     | 69.8    | 2.1            | 0.8          |

Table 14: Config 6: X2 fully observed. True values are  $\beta_1 = -0.11$ ,  $\beta_2 = 0.03$ ,  $\sqrt{\psi_{00}} = 0.09$ ,  $\sqrt{\psi_{11}} = 0.02$ .

|                           | Full    | JM-jomo | FCS-GLM | FCS-2stageREML | FCS-2stageMM |
|---------------------------|---------|---------|---------|----------------|--------------|
| $\beta^{(1)}$ est         | -0.1101 | -0.1087 | -0.1103 | -0.1091        | -0.1091      |
| $\beta^{(1)}$ rbias (%)   | 0.1     | -1.2    | 0.3     | -0.8           | -0.8         |
| $\beta^{(1)}$ model se    | 0.0047  | 0.0065  | 0.0047  | 0.0059         | 0.0058       |
| $\beta^{(1)}$ emp se      | 0.0048  | 0.0057  | 0.0057  | 0.0057         | 0.0058       |
| $\beta^{(1)}$ 95% cover   | 93.8    | 96.4    | 88.6    | 93.5           | 92.0         |
| $\beta^{(1)}$ rmse        | 0.0048  | 0.0058  | 0.0057  | 0.0057         | 0.0059       |
| $\beta^{(2)}$ est         | 0.0301  | 0.0301  | 0.0300  | 0.0300         | 0.0300       |
| $\beta^{(2)}$ rbias (%)   | 0.2     | 0.3     | 0.1     | 0.0            | -0.0         |
| $\beta^{(2)}$ model se    | 0.0029  | 0.0037  | 0.0031  | 0.0036         | 0.0035       |
| $\beta^{(2)}$ emp se      | 0.0030  | 0.0033  | 0.0032  | 0.0032         | 0.0034       |
| $\beta^{(2)}$ 95% cover   | 94.2    | 95.2    | 93.8    | 95.6           | 95.8         |
| $\beta^{(2)}$ rmse        | 0.0030  | 0.0033  | 0.0032  | 0.0032         | 0.0034       |
| $\sqrt{\psi_0}$ est       | 0.0859  | 0.0926  | 0.0780  | 0.0864         | 0.0859       |
| $\sqrt{\psi_0}$ rbias (%) | -2.1    | 5.5     | -11.1   | -1.5           | -2.1         |
| $\sqrt{\psi_0}$ rmse      | 0.0154  | 0.0151  | 0.0173  | 0.0156         | 0.0150       |
| $\sqrt{\psi_1}$ est       | 0.0193  | 0.0218  | 0.0151  | 0.0196         | 0.0195       |
| $\sqrt{\psi_1}$ rbias (%) | -3.7    | 9.0     | -24.3   | -1.8           | -2.6         |
| $\sqrt{\psi_1}$ rmse      | 0.0041  | 0.0041  | 0.0065  | 0.0047         | 0.0046       |
| time                      |         | 4.6     | 3.0     | 0.2            | 0.1          |

Table 15: Config 7: X1 fully observed. True values are  $\beta_1 = -0.11$ ,  $\beta_2 = 0.03$ ,  $\sqrt{\psi_{00}} = 0.09$ ,  $\sqrt{\psi_{11}} = 0.02$ .

|                           | Full    | JM-jomo | FCS-GLM | FCS-2stageREML | FCS-2stageMM |
|---------------------------|---------|---------|---------|----------------|--------------|
| $\beta^{(1)}$ est         | -0.1101 | -0.1101 | -0.1102 | -0.1101        | -0.1101      |
| $\beta^{(1)}$ rbias (%)   | 0.1     | 0.1     | 0.2     | 0.1            | 0.1          |
| $\beta^{(1)}$ model se    | 0.0047  | 0.0047  | 0.0047  | 0.0047         | 0.0047       |
| $\beta^{(1)}$ emp se      | 0.0048  | 0.0048  | 0.0048  | 0.0048         | 0.0048       |
| $\beta^{(1)}$ 95% cover   | 93.8    | 94.2    | 94.2    | 94.2           | 94.0         |
| $\beta^{(1)}$ rmse        | 0.0048  | 0.0048  | 0.0048  | 0.0048         | 0.0048       |
| $\beta^{(2)}$ est         | 0.0301  | 0.0297  | 0.0298  | 0.0296         | 0.0296       |
| $\beta^{(2)}$ rbias (%)   | 0.2     | -0.9    | -0.7    | -1.4           | -1.2         |
| $\beta^{(2)}$ model se    | 0.0029  | 0.0060  | 0.0041  | 0.0046         | 0.0041       |
| $\beta^{(2)}$ emp se      | 0.0030  | 0.0043  | 0.0040  | 0.0041         | 0.0041       |
| $\beta^{(2)}$ 95% cover   | 94.2    | 98.2    | 95.8    | 96.4           | 95.0         |
| $\beta^{(2)}$ rmse        | 0.0030  | 0.0043  | 0.0040  | 0.0041         | 0.0041       |
| $\sqrt{\psi_0}$ est       | 0.0859  | 0.0859  | 0.0856  | 0.0857         | 0.0856       |
| $\sqrt{\psi_0}$ rbias (%) | -2.1    | -2.1    | -2.5    | -2.3           | -2.4         |
| $\sqrt{\psi_0}$ rmse      | 0.0154  | 0.0154  | 0.0154  | 0.0154         | 0.0154       |
| $\sqrt{\psi_1}$ est       | 0.0193  | 0.0192  | 0.0192  | 0.0192         | 0.0192       |
| $\sqrt{\psi_1}$ rbias (%) | -3.7    | -3.8    | -4.1    | -4.0           | -4.1         |
| $\sqrt{\psi_1}$ rmse      | 0.0041  | 0.0041  | 0.0041  | 0.0041         | 0.0041       |
| time                      |         | 7.0     | 17.6    | 0.2            | 0.1          |

Table 16: Config 8: MAR mechanism. True values are  $\beta_1 = -0.11$ ,  $\beta_2 = 0.03$ ,  $\sqrt{\psi_{00}} = 0.09$ ,  $\sqrt{\psi_{11}} = 0.02$ .

|                           | Full    | JM-jomo | FCS-GLM | FCS-2stageREML | FCS-2stageMM |
|---------------------------|---------|---------|---------|----------------|--------------|
| $\beta^{(1)}$ est         | -0.1101 | -0.1085 | -0.1100 | -0.1086        | -0.1086      |
| $\beta^{(1)}$ rbias (%)   | 0.1     | -1.4    | -0.0    | -1.3           | -1.3         |
| $\beta^{(1)}$ model se    | 0.0047  | 0.0067  | 0.0047  | 0.0062         | 0.0060       |
| $\beta^{(1)}$ emp se      | 0.0048  | 0.0058  | 0.0056  | 0.0059         | 0.0058       |
| $\beta^{(1)}$ 95% cover   | 93.8    | 97.0    | 89.7    | 94.9           | 94.0         |
| $\beta^{(1)}$ rmse        | 0.0048  | 0.0060  | 0.0056  | 0.0061         | 0.0060       |
| $\beta^{(2)}$ est         | 0.0301  | 0.0299  | 0.0298  | 0.0296         | 0.0297       |
| $\beta^{(2)}$ rbias (%)   | 0.2     | -0.4    | -0.6    | -1.3           | -1.1         |
| $\beta^{(2)}$ model se    | 0.0029  | 0.0069  | 0.0045  | 0.0054         | 0.0052       |
| $\beta^{(2)}$ emp se      | 0.0030  | 0.0046  | 0.0046  | 0.0046         | 0.0047       |
| $\beta^{(2)}$ 95% cover   | 94.2    | 98.6    | 94.1    | 96.8           | 94.8         |
| $\beta^{(2)}$ rmse        | 0.0030  | 0.0046  | 0.0046  | 0.0046         | 0.0047       |
| $\sqrt{\psi_0}$ est       | 0.0859  | 0.0937  | 0.0775  | 0.0868         | 0.0866       |
| $\sqrt{\psi_0}$ rbias (%) | -2.1    | 6.8     | -11.7   | -1.0           | -1.3         |
| $\sqrt{\psi_0}$ rmse      | 0.0154  | 0.0151  | 0.0170  | 0.0143         | 0.0144       |
| $\sqrt{\psi_1}$ est       | 0.0193  | 0.0222  | 0.0147  | 0.0199         | 0.0197       |
| $\sqrt{\psi_1}$ rbias (%) | -3.7    | 10.9    | -26.6   | -0.7           | -1.6         |
| $\sqrt{\psi_1}$ rmse      | 0.0041  | 0.0043  | 0.0068  | 0.0044         | 0.0044       |
| time                      |         | 7.7     | 100.4   | 2.2            | 0.9          |

Table 17: Config 9: Random slope. True values are  $\beta_1 = -0.11$ ,  $\beta_2 = 0.03$ ,  $\sqrt{\psi_{00}} = 0.09$ ,  $\sqrt{\psi_{11}} = 0.02$ .

|                           | Full    | JM-jomo | FCS-GLM | FCS-2stageREML | FCS-2stageMM |
|---------------------------|---------|---------|---------|----------------|--------------|
| $\beta^{(1)}$ est         | -0.1102 | -0.1087 | -0.1099 | -0.1090        | -0.1092      |
| $\beta^{(1)}$ rbias (%)   | 0.2     | -1.2    | -0.1    | -0.9           | -0.7         |
| $\beta^{(1)}$ model se    | 0.0047  | 0.0067  | 0.0047  | 0.0059         | 0.0059       |
| $\beta^{(1)}$ emp se      | 0.0048  | 0.0058  | 0.0057  | 0.0058         | 0.0058       |
| $\beta^{(1)}$ 95% cover   | 94.0    | 97.2    | 91.1    | 95.0           | 94.0         |
| $\beta^{(1)}$ rmse        | 0.0048  | 0.0060  | 0.0057  | 0.0059         | 0.0059       |
| $\beta^{(2)}$ est         | 0.0296  | 0.0295  | 0.0291  | 0.0290         | 0.0291       |
| $\beta^{(2)}$ rbias (%)   | -1.5    | -1.7    | -2.9    | -3.4           | -3.0         |
| $\beta^{(2)}$ model se    | 0.0062  | 0.0087  | 0.0071  | 0.0085         | 0.0079       |
| $\beta^{(2)}$ emp se      | 0.0060  | 0.0082  | 0.0077  | 0.0078         | 0.0077       |
| $\beta^{(2)}$ 95% cover   | 93.4    | 96.0    | 90.3    | 96.0           | 94.8         |
| $\beta^{(2)}$ rmse        | 0.0060  | 0.0082  | 0.0077  | 0.0078         | 0.0078       |
| $\sqrt{\psi_0}$ est       | 0.0857  | 0.0953  | 0.0789  | 0.0880         | 0.0869       |
| $\sqrt{\psi_0}$ rbias (%) | -2.4    | 8.6     | -10.1   | 0.3            | -0.9         |
| $\sqrt{\psi_0}$ rmse      | 0.0156  | 0.0154  | 0.0168  | 0.0149         | 0.0152       |
| $\sqrt{\psi_1}$ est       | 0.0193  | 0.0224  | 0.0152  | 0.0198         | 0.0194       |
| $\sqrt{\psi_1}$ rbias (%) | -3.7    | 12.1    | -24.0   | -1.2           | -2.9         |
| $\sqrt{\psi_1}$ rmse      | 0.0041  | 0.0044  | 0.0065  | 0.0046         | 0.0047       |
| time                      |         | 7.7     | 122.2   | 2.2            | 0.9          |

Table 18: Config 10: Few clusters. True values are  $\beta_1 = -0.11$ ,  $\beta_2 = 0.03$ ,  $\sqrt{\psi_{00}} = 0.09$ ,  $\sqrt{\psi_{11}} = 0.02$ .

|                           | Full    | JM-jomo | FCS-GLM | FCS-2stageREML | FCS-2stageMM |
|---------------------------|---------|---------|---------|----------------|--------------|
| $\beta^{(1)}$ est         | -0.1100 | -0.1075 | -0.1098 | -0.1090        | -0.1093      |
| $\beta^{(1)}$ rbias (%)   | 0.0     | -2.3    | -0.2    | -0.9           | -0.6         |
| $\beta^{(1)}$ model se    | 0.0069  | 0.0109  | 0.0074  | 0.0088         | 0.0082       |
| $\beta^{(1)}$ emp se      | 0.0072  | 0.0085  | 0.0085  | 0.0085         | 0.0085       |
| $\beta^{(1)}$ 95% cover   | 92.2    | 98.4    | 90.5    | 95.4           | 93.4         |
| $\beta^{(1)}$ rmse        | 0.0072  | 0.0089  | 0.0085  | 0.0086         | 0.0086       |
| $\beta^{(2)}$ est         | 0.0298  | 0.0294  | 0.0293  | 0.0293         | 0.0293       |
| $\beta^{(2)}$ rbias (%)   | -0.6    | -2.1    | -2.4    | -2.4           | -2.3         |
| $\beta^{(2)}$ model se    | 0.0048  | 0.0108  | 0.0077  | 0.0088         | 0.0079       |
| $\beta^{(2)}$ emp se      | 0.0045  | 0.0077  | 0.0069  | 0.0071         | 0.0069       |
| $\beta^{(2)}$ 95% cover   | 95.4    | 97.8    | 95.8    | 97.8           | 95.6         |
| $\beta^{(2)}$ rmse        | 0.0045  | 0.0078  | 0.0069  | 0.0072         | 0.0070       |
| $\sqrt{\psi_0}$ est       | 0.0859  | 0.0998  | 0.0791  | 0.0860         | 0.0839       |
| $\sqrt{\psi_0}$ rbias (%) | -2.1    | 13.7    | -9.9    | -2.0           | -4.4         |
| $\sqrt{\psi_0}$ rmse      | 0.0236  | 0.0247  | 0.0236  | 0.0221         | 0.0229       |
| $\sqrt{\psi_1}$ est       | 0.0191  | 0.0245  | 0.0154  | 0.0192         | 0.0182       |
| $\sqrt{\psi_1}$ rbias (%) | -4.4    | 22.4    | -23.2   | -4.2           | -8.8         |
| $\sqrt{\psi_1}$ rmse      | 0.0065  | 0.0075  | 0.0080  | 0.0066         | 0.0068       |
| time                      |         | 2.6     | 37.8    | 1.0            | 0.3          |



Table 19: Config 11: Few individuals. True values are  $\beta_1 = -0.11$ ,  $\beta_2 = 0.03$ ,  $\sqrt{\psi_{00}} = 0.09$ ,  $\sqrt{\psi_{11}} = 0.02$ .

|                           | Full    | JM-jomo | FCS-GLM | FCS-2stageREML | FCS-2stageMM |
|---------------------------|---------|---------|---------|----------------|--------------|
| $\beta^{(1)}$ est         | -0.1094 | -0.1073 | -0.1090 | -0.1077        | -0.1076      |
| $\beta^{(1)}$ rbias (%)   | -0.5    | -2.5    | -0.9    | -2.1           | -2.2         |
| $\beta^{(1)}$ model se    | 0.0053  | 0.0077  | 0.0057  | 0.0071         | 0.0072       |
| $\beta^{(1)}$ emp se      | 0.0057  | 0.0066  | 0.0066  | 0.0066         | 0.0067       |
| $\beta^{(1)}$ 95% cover   | 90.6    | 96.8    | 88.7    | 91.8           | 94.8         |
| $\beta^{(1)}$ rmse        | 0.0057  | 0.0071  | 0.0067  | 0.0070         | 0.0072       |
| $\beta^{(2)}$ est         | 0.0296  | 0.0295  | 0.0293  | 0.0281         | 0.0291       |
| $\beta^{(2)}$ rbias (%)   | -1.4    | -1.6    | -2.4    | -6.5           | -2.9         |
| $\beta^{(2)}$ model se    | 0.0041  | 0.0083  | 0.0063  | 0.0075         | 0.0068       |
| $\beta^{(2)}$ emp se      | 0.0042  | 0.0068  | 0.0065  | 0.0058         | 0.0059       |
| $\beta^{(2)}$ 95% cover   | 93.0    | 97.0    | 93.9    | 100.0          | 97.4         |
| $\beta^{(2)}$ rmse        | 0.0043  | 0.0069  | 0.0066  | 0.0061         | 0.0060       |
| $\sqrt{\psi_0}$ est       | 0.0849  | 0.0949  | 0.0765  | 0.0871         | 0.0883       |
| $\sqrt{\psi_0}$ rbias (%) | -3.2    | 8.1     | -12.8   | -0.7           | 0.7          |
| $\sqrt{\psi_0}$ rmse      | 0.0179  | 0.0178  | 0.0201  | 0.0186         | 0.0178       |
| $\sqrt{\psi_1}$ est       | 0.0190  | 0.0230  | 0.0148  | 0.0208         | 0.0211       |
| $\sqrt{\psi_1}$ rbias (%) | -4.9    | 15.2    | -26.0   | 3.8            | 5.5          |
| $\sqrt{\psi_1}$ rmse      | 0.0055  | 0.0057  | 0.0074  | 0.0060         | 0.0058       |
| time                      |         | 3.8     | 55.1    | 0.6            | 0.3          |

Table 20: Config 12: Very few individuals. True values are  $\beta_1 = -0.11$ ,  $\beta_2 = 0.03$ ,  $\sqrt{\psi_{00}} = 0.09$ ,  $\sqrt{\psi_{11}} = 0.02$ .

|                           | Full    | JM-jomo | FCS-GLM | FCS-2stageREML | FCS-2stageMM |
|---------------------------|---------|---------|---------|----------------|--------------|
| $\beta^{(1)}$ est         | -0.1102 | -0.1073 | -0.1099 | -0.1060        | -0.1062      |
| $\beta^{(1)}$ rbias (%)   | 0.2     | -2.4    | -0.1    | -3.6           | -3.5         |
| $\beta^{(1)}$ model se    | 0.0064  | 0.0093  | 0.0072  | 0.0098         | 0.0098       |
| $\beta^{(1)}$ emp se      | 0.0063  | 0.0083  | 0.0079  | 0.0081         | 0.0088       |
| $\beta^{(1)}$ 95% cover   | 93.8    | 96.6    | 92.4    | 97.5           | 96.2         |
| $\beta^{(1)}$ rmse        | 0.0063  | 0.0087  | 0.0079  | 0.0090         | 0.0096       |
| $\beta^{(2)}$ est         | 0.0297  | 0.0292  | 0.0289  | 0.0288         | 0.0286       |
| $\beta^{(2)}$ rbias (%)   | -1.1    | -2.7    | -3.6    | -3.8           | -4.7         |
| $\beta^{(2)}$ model se    | 0.0058  | 0.0107  | 0.0092  | 0.0100         | 0.0094       |
| $\beta^{(2)}$ emp se      | 0.0056  | 0.0093  | 0.0086  | 0.0089         | 0.0083       |
| $\beta^{(2)}$ 95% cover   | 94.6    | 96.6    | 96.2    | 96.7           | 97.7         |
| $\beta^{(2)}$ rmse        | 0.0057  | 0.0093  | 0.0086  | 0.0090         | 0.0084       |
| $\sqrt{\psi_0}$ est       | 0.0861  | 0.0972  | 0.0780  | 0.0993         | 0.0987       |
| $\sqrt{\psi_0}$ rbias (%) | -1.8    | 10.7    | -11.1   | 13.2           | 12.5         |
| $\sqrt{\psi_0}$ rmse      | 0.0228  | 0.0214  | 0.0225  | 0.0262         | 0.0269       |
| $\sqrt{\psi_1}$ est       | 0.0193  | 0.0241  | 0.0153  | 0.0257         | 0.0255       |
| $\sqrt{\psi_1}$ rbias (%) | -3.3    | 20.7    | -23.5   | 28.4           | 27.4         |
| $\sqrt{\psi_1}$ rmse      | 0.0076  | 0.0076  | 0.0082  | 0.0100         | 0.0101       |
| time                      |         | 1.9     | 32.6    | 0.9            | 0.4          |

Table 21: Config 13: Strong ICC. True values are  $\beta_1 = -0.11$ ,  $\beta_2 = 0.03$ ,  $\sqrt{\psi_{00}} = 0.09$ ,  $\sqrt{\psi_{11}} = 0.02$ .

|                           | Full    | JM-jomo | FCS-GLM | FCS-2stageREML | FCS-2stageMM |
|---------------------------|---------|---------|---------|----------------|--------------|
| $\beta^{(1)}$ est         | -0.1102 | -0.1083 | -0.1098 | -0.1086        | -0.1088      |
| $\beta^{(1)}$ rbias (%)   | 0.1     | -1.5    | -0.2    | -1.2           | -1.1         |
| $\beta^{(1)}$ model se    | 0.0047  | 0.0066  | 0.0047  | 0.0060         | 0.0059       |
| $\beta^{(1)}$ emp se      | 0.0048  | 0.0058  | 0.0057  | 0.0058         | 0.0058       |
| $\beta^{(1)}$ 95% cover   | 94.4    | 96.6    | 91.2    | 94.2           | 94.4         |
| $\beta^{(1)}$ rmse        | 0.0048  | 0.0061  | 0.0057  | 0.0060         | 0.0059       |
| $\beta^{(2)}$ est         | 0.0301  | 0.0299  | 0.0294  | 0.0297         | 0.0299       |
| $\beta^{(2)}$ rbias (%)   | 0.5     | -0.4    | -1.8    | -0.9           | -0.4         |
| $\beta^{(2)}$ model se    | 0.0029  | 0.0069  | 0.0046  | 0.0055         | 0.0051       |
| $\beta^{(2)}$ emp se      | 0.0030  | 0.0049  | 0.0044  | 0.0047         | 0.0045       |
| $\beta^{(2)}$ 95% cover   | 94.4    | 97.6    | 95.2    | 96.2           | 95.2         |
| $\beta^{(2)}$ rmse        | 0.0030  | 0.0049  | 0.0045  | 0.0047         | 0.0045       |
| $\sqrt{\psi_0}$ est       | 0.0859  | 0.0995  | 0.0855  | 0.0932         | 0.0925       |
| $\sqrt{\psi_0}$ rbias (%) | -2.1    | 13.4    | -2.5    | 6.2            | 5.5          |
| $\sqrt{\psi_0}$ rmse      | 0.0154  | 0.0184  | 0.0143  | 0.0157         | 0.0155       |
| $\sqrt{\psi_1}$ est       | 0.0193  | 0.0223  | 0.0152  | 0.0198         | 0.0194       |
| $\sqrt{\psi_1}$ rbias (%) | -3.6    | 11.7    | -24.0   | -0.9           | -2.9         |
| $\sqrt{\psi_1}$ rmse      | 0.0041  | 0.0043  | 0.0065  | 0.0046         | 0.0048       |
| time                      |         | 7.7     | 85.5    | 2.1            | 0.9          |

Table 22: Config 14: Weak ICC. True values are  $\beta_1 = -0.11$ ,  $\beta_2 = 0.03$ ,  $\sqrt{\psi_{00}} = 0.09$ ,  $\sqrt{\psi_{11}} = 0.02$ .

|                           | Full    | JM-jomo | FCS-GLM | FCS-2stageREML | FCS-2stageMM |
|---------------------------|---------|---------|---------|----------------|--------------|
| $\beta^{(1)}$ est         | -0.1101 | -0.1086 | -0.1100 | -0.1089        | -0.1091      |
| $\beta^{(1)}$ rbias (%)   | 0.1     | -1.3    | -0.0    | -1.0           | -0.8         |
| $\beta^{(1)}$ model se    | 0.0047  | 0.0067  | 0.0047  | 0.0059         | 0.0059       |
| $\beta^{(1)}$ emp se      | 0.0048  | 0.0057  | 0.0057  | 0.0058         | 0.0058       |
| $\beta^{(1)}$ 95% cover   | 94.0    | 96.8    | 89.7    | 95.2           | 94.8         |
| $\beta^{(1)}$ rmse        | 0.0048  | 0.0059  | 0.0057  | 0.0059         | 0.0059       |
| $\beta^{(2)}$ est         | 0.0300  | 0.0297  | 0.0296  | 0.0294         | 0.0296       |
| $\beta^{(2)}$ rbias (%)   | 0.1     | -1.1    | -1.2    | -2.1           | -1.4         |
| $\beta^{(2)}$ model se    | 0.0029  | 0.0067  | 0.0045  | 0.0054         | 0.0049       |
| $\beta^{(2)}$ emp se      | 0.0029  | 0.0049  | 0.0042  | 0.0043         | 0.0043       |
| $\beta^{(2)}$ 95% cover   | 94.4    | 98.6    | 96.2    | 97.4           | 96.6         |
| $\beta^{(2)}$ rmse        | 0.0029  | 0.0049  | 0.0042  | 0.0044         | 0.0044       |
| $\sqrt{\psi_0}$ est       | 0.0859  | 0.0920  | 0.0754  | 0.0847         | 0.0840       |
| $\sqrt{\psi_0}$ rbias (%) | -2.1    | 4.8     | -14.1   | -3.4           | -4.3         |
| $\sqrt{\psi_0}$ rmse      | 0.0154  | 0.0142  | 0.0190  | 0.0153         | 0.0155       |
| $\sqrt{\psi_1}$ est       | 0.0193  | 0.0224  | 0.0151  | 0.0198         | 0.0194       |
| $\sqrt{\psi_1}$ rbias (%) | -3.7    | 12.0    | -24.5   | -1.2           | -3.0         |
| $\sqrt{\psi_1}$ rmse      | 0.0041  | 0.0044  | 0.0066  | 0.0046         | 0.0047       |
| time                      |         | 7.7     | 122.4   | 2.3            | 0.9          |

Table 23: Config 15: Stronger correlation SigmaV. True values are  $\beta_1 = -0.11$ ,  $\beta_2 = 0.03$ ,  $\sqrt{\psi_{00}} = 0.09$ ,  $\sqrt{\psi_{11}} = 0.02$ .

|                           | Full    | JM-jomo | FCS-GLM | FCS-2stageREML | FCS-2stageMM |
|---------------------------|---------|---------|---------|----------------|--------------|
| $\beta^{(1)}$ est         | -0.1101 | -0.1087 | -0.1100 | -0.1089        | -0.1090      |
| $\beta^{(1)}$ rbias (%)   | 0.1     | -1.2    | 0.0     | -1.0           | -0.9         |
| $\beta^{(1)}$ model se    | 0.0047  | 0.0066  | 0.0047  | 0.0059         | 0.0059       |
| $\beta^{(1)}$ emp se      | 0.0048  | 0.0056  | 0.0057  | 0.0058         | 0.0058       |
| $\beta^{(1)}$ 95% cover   | 94.0    | 96.2    | 90.9    | 95.0           | 95.0         |
| $\beta^{(1)}$ rmse        | 0.0048  | 0.0058  | 0.0057  | 0.0059         | 0.0059       |
| $\beta^{(2)}$ est         | 0.0300  | 0.0299  | 0.0298  | 0.0296         | 0.0298       |
| $\beta^{(2)}$ rbias (%)   | 0.1     | -0.2    | -0.7    | -1.2           | -0.7         |
| $\beta^{(2)}$ model se    | 0.0029  | 0.0070  | 0.0045  | 0.0054         | 0.0049       |
| $\beta^{(2)}$ emp se      | 0.0030  | 0.0049  | 0.0043  | 0.0045         | 0.0044       |
| $\beta^{(2)}$ 95% cover   | 94.4    | 97.8    | 94.3    | 97.0           | 95.4         |
| $\beta^{(2)}$ rmse        | 0.0030  | 0.0049  | 0.0043  | 0.0045         | 0.0044       |
| $\sqrt{\psi_0}$ est       | 0.0859  | 0.0938  | 0.0777  | 0.0864         | 0.0858       |
| $\sqrt{\psi_0}$ rbias (%) | -2.1    | 6.8     | -11.5   | -1.5           | -2.2         |
| $\sqrt{\psi_0}$ rmse      | 0.0154  | 0.0150  | 0.0175  | 0.0149         | 0.0151       |
| $\sqrt{\psi_1}$ est       | 0.0193  | 0.0222  | 0.0152  | 0.0197         | 0.0194       |
| $\sqrt{\psi_1}$ rbias (%) | -3.7    | 11.1    | -24.1   | -1.3           | -2.8         |
| $\sqrt{\psi_1}$ rmse      | 0.0041  | 0.0043  | 0.0066  | 0.0046         | 0.0048       |
| time                      |         | 7.7     | 103.2   | 2.2            | 0.9          |

Table 24: Config 16: Stronger correlation (X1, X3). True values are  $\beta_1 = -0.11$ ,  $\beta_2 = 0.03$ ,  $\sqrt{\psi_{00}} = 0.09$ ,  $\sqrt{\psi_{11}} = 0.02$ .

|                           | Full    | JM-jomo | FCS-GLM | FCS-2stageREML | FCS-2stageMM |
|---------------------------|---------|---------|---------|----------------|--------------|
| $\beta^{(1)}$ est         | -0.1101 | -0.1087 | -0.1099 | -0.1091        | -0.1091      |
| $\beta^{(1)}$ rbias (%)   | 0.1     | -1.2    | -0.1    | -0.9           | -0.8         |
| $\beta^{(1)}$ model se    | 0.0047  | 0.0064  | 0.0047  | 0.0058         | 0.0058       |
| $\beta^{(1)}$ emp se      | 0.0048  | 0.0056  | 0.0056  | 0.0057         | 0.0057       |
| $\beta^{(1)}$ 95% cover   | 94.0    | 96.6    | 91.8    | 95.2           | 95.0         |
| $\beta^{(1)}$ rmse        | 0.0048  | 0.0058  | 0.0056  | 0.0058         | 0.0058       |
| $\beta^{(2)}$ est         | 0.0301  | 0.0298  | 0.0297  | 0.0296         | 0.0297       |
| $\beta^{(2)}$ rbias (%)   | 0.2     | -0.8    | -1.0    | -1.5           | -1.0         |
| $\beta^{(2)}$ model se    | 0.0029  | 0.0069  | 0.0045  | 0.0054         | 0.0048       |
| $\beta^{(2)}$ emp se      | 0.0030  | 0.0050  | 0.0042  | 0.0044         | 0.0043       |
| $\beta^{(2)}$ 95% cover   | 94.2    | 98.0    | 93.8    | 97.4           | 95.4         |
| $\beta^{(2)}$ rmse        | 0.0030  | 0.0050  | 0.0042  | 0.0044         | 0.0043       |
| $\sqrt{\psi_0}$ est       | 0.0859  | 0.0933  | 0.0801  | 0.0878         | 0.0873       |
| $\sqrt{\psi_0}$ rbias (%) | -2.1    | 6.4     | -8.8    | 0.0            | -0.5         |
| $\sqrt{\psi_0}$ rmse      | 0.0154  | 0.0148  | 0.0161  | 0.0146         | 0.0146       |
| $\sqrt{\psi_1}$ est       | 0.0192  | 0.0219  | 0.0155  | 0.0197         | 0.0194       |
| $\sqrt{\psi_1}$ rbias (%) | -3.8    | 9.4     | -22.4   | -1.6           | -2.9         |
| $\sqrt{\psi_1}$ rmse      | 0.0041  | 0.0041  | 0.0063  | 0.0045         | 0.0046       |
| time                      |         | 7.6     | 103.2   | 2.2            | 0.9          |

Table 25: Config 18: Higher correlation Psi. True values are  $\beta_1 = -0.11$ ,  $\beta_2 = 0.03$ ,  $\sqrt{\psi_{00}} = 0.09$ ,  $\sqrt{\psi_{11}} = 0.02$ .

|                           | Full    | JM-jomo | FCS-GLM | FCS-2stageREML | FCS-2stageMM |
|---------------------------|---------|---------|---------|----------------|--------------|
| $\beta^{(1)}$ est         | -0.1100 | -0.1086 | -0.1099 | -0.1088        | -0.1089      |
| $\beta^{(1)}$ rbias (%)   | 0.0     | -1.3    | -0.1    | -1.1           | -1.0         |
| $\beta^{(1)}$ model se    | 0.0047  | 0.0067  | 0.0047  | 0.0060         | 0.0059       |
| $\beta^{(1)}$ emp se      | 0.0048  | 0.0058  | 0.0057  | 0.0058         | 0.0058       |
| $\beta^{(1)}$ 95% cover   | 93.8    | 96.6    | 88.9    | 93.8           | 94.4         |
| $\beta^{(1)}$ rmse        | 0.0048  | 0.0060  | 0.0057  | 0.0059         | 0.0059       |
| $\beta^{(2)}$ est         | 0.0301  | 0.0300  | 0.0293  | 0.0293         | 0.0295       |
| $\beta^{(2)}$ rbias (%)   | 0.2     | -0.1    | -2.2    | -2.4           | -1.7         |
| $\beta^{(2)}$ model se    | 0.0029  | 0.0069  | 0.0046  | 0.0054         | 0.0050       |
| $\beta^{(2)}$ emp se      | 0.0030  | 0.0051  | 0.0042  | 0.0044         | 0.0044       |
| $\beta^{(2)}$ 95% cover   | 94.2    | 97.8    | 94.0    | 97.0           | 97.0         |
| $\beta^{(2)}$ rmse        | 0.0030  | 0.0051  | 0.0042  | 0.0045         | 0.0044       |
| $\sqrt{\psi_0}$ est       | 0.0862  | 0.0999  | 0.0858  | 0.0927         | 0.0921       |
| $\sqrt{\psi_0}$ rbias (%) | -1.8    | 13.9    | -2.3    | 5.7            | 4.9          |
| $\sqrt{\psi_0}$ rmse      | 0.0153  | 0.0189  | 0.0140  | 0.0156         | 0.0154       |
| $\sqrt{\psi_1}$ est       | 0.0192  | 0.0223  | 0.0151  | 0.0198         | 0.0195       |
| $\sqrt{\psi_1}$ rbias (%) | -3.8    | 11.3    | -24.5   | -1.0           | -2.7         |
| $\sqrt{\psi_1}$ rmse      | 0.0040  | 0.0042  | 0.0066  | 0.0046         | 0.0047       |
| time                      |         | 7.7     | 101.4   | 2.2            | 0.9          |

Table 26: Config 19: Probit. True values are  $\beta_1 = -0.11$ ,  $\beta_2 = 0.03$ ,  $\sqrt{\psi_{00}} = 0.09$ ,  $\sqrt{\psi_{11}} = 0.02$ .

|                           | Full    | JM-jomo | FCS-GLM | FCS-2stageREML | FCS-2stageMM |
|---------------------------|---------|---------|---------|----------------|--------------|
| $\beta^{(1)}$ est         | -0.1101 | -0.1085 | -0.1100 | -0.1089        | -0.1090      |
| $\beta^{(1)}$ rbias (%)   | 0.1     | -1.4    | 0.0     | -1.0           | -0.9         |
| $\beta^{(1)}$ model se    | 0.0047  | 0.0067  | 0.0047  | 0.0059         | 0.0059       |
| $\beta^{(1)}$ emp se      | 0.0048  | 0.0058  | 0.0056  | 0.0057         | 0.0058       |
| $\beta^{(1)}$ 95% cover   | 93.8    | 96.6    | 90.6    | 94.0           | 94.6         |
| $\beta^{(1)}$ rmse        | 0.0048  | 0.0060  | 0.0056  | 0.0058         | 0.0058       |
| $\beta^{(2)}$ est         | 0.0300  | 0.0297  | 0.0296  | 0.0295         | 0.0296       |
| $\beta^{(2)}$ rbias (%)   | -0.1    | -0.9    | -1.3    | -1.5           | -1.3         |
| $\beta^{(2)}$ model se    | 0.0029  | 0.0070  | 0.0047  | 0.0056         | 0.0051       |
| $\beta^{(2)}$ emp se      | 0.0030  | 0.0049  | 0.0045  | 0.0047         | 0.0046       |
| $\beta^{(2)}$ 95% cover   | 94.6    | 98.6    | 95.2    | 96.2           | 96.4         |
| $\beta^{(2)}$ rmse        | 0.0030  | 0.0049  | 0.0045  | 0.0047         | 0.0046       |
| $\sqrt{\psi_0}$ est       | 0.0859  | 0.0944  | 0.0782  | 0.0871         | 0.0862       |
| $\sqrt{\psi_0}$ rbias (%) | -2.1    | 7.6     | -10.9   | -0.8           | -1.7         |
| $\sqrt{\psi_0}$ rmse      | 0.0154  | 0.0152  | 0.0171  | 0.0147         | 0.0150       |
| $\sqrt{\psi_1}$ est       | 0.0193  | 0.0224  | 0.0151  | 0.0198         | 0.0194       |
| $\sqrt{\psi_1}$ rbias (%) | -3.7    | 12.1    | -24.4   | -0.9           | -3.0         |
| $\sqrt{\psi_1}$ rmse      | 0.0041  | 0.0044  | 0.0066  | 0.0046         | 0.0048       |
| time                      |         | 7.7     | 122.4   | 2.3            | 0.9          |



Table 27: Config 20: Few clusters. True values are  $\beta_1 = -0.11$ ,  $\beta_2 = 0.03$ ,  $\sqrt{\psi_{00}} = 0.09$ ,  $\sqrt{\psi_{11}} = 0.02$ .

|                           | Full    | JM-jomo | FCS-GLM | FCS-2stageREML | FCS-2stageMM |
|---------------------------|---------|---------|---------|----------------|--------------|
| $\beta^{(1)}$ est         | -0.1103 | -0.1042 | -0.1089 | -0.1083        | -0.1087      |
| $\beta^{(1)}$ rbias (%)   | 0.2     | -5.2    | -1.0    | -1.6           | -1.2         |
| $\beta^{(1)}$ model se    | 0.0093  | 0.0192  | 0.0110  | 0.0127         | 0.0117       |
| $\beta^{(1)}$ emp se      | 0.0091  | 0.0138  | 0.0115  | 0.0121         | 0.0118       |
| $\beta^{(1)}$ 95% cover   | 92.2    | 97.4    | 91.0    | 93.8           | 91.1         |
| $\beta^{(1)}$ rmse        | 0.0091  | 0.0149  | 0.0116  | 0.0122         | 0.0118       |
| $\beta^{(2)}$ est         | 0.0299  | 0.0285  | 0.0283  | 0.0289         | 0.0292       |
| $\beta^{(2)}$ rbias (%)   | -0.3    | -5.1    | -5.6    | -3.5           | -2.6         |
| $\beta^{(2)}$ model se    | 0.0067  | 0.0187  | 0.0116  | 0.0153         | 0.0121       |
| $\beta^{(2)}$ emp se      | 0.0067  | 0.0145  | 0.0108  | 0.0116         | 0.0111       |
| $\beta^{(2)}$ 95% cover   | 95.8    | 96.6    | 96.1    | 96.8           | 94.0         |
| $\beta^{(2)}$ rmse        | 0.0067  | 0.0145  | 0.0110  | 0.0117         | 0.0111       |
| $\sqrt{\psi_0}$ est       | 0.0802  | 0.1065  | 0.0757  | 0.0815         | 0.0781       |
| $\sqrt{\psi_0}$ rbias (%) | -8.7    | 21.4    | -13.7   | -7.1           | -11.0        |
| $\sqrt{\psi_0}$ rmse      | 0.0338  | 0.0380  | 0.0328  | 0.0309         | 0.0311       |
| $\sqrt{\psi_1}$ est       | 0.0176  | 0.0274  | 0.0151  | 0.0183         | 0.0165       |
| $\sqrt{\psi_1}$ rbias (%) | -12.1   | 36.9    | -24.5   | -8.7           | -17.3        |
| $\sqrt{\psi_1}$ rmse      | 0.0093  | 0.0124  | 0.0098  | 0.0089         | 0.0093       |
| time                      |         | 1.2     | 14.8    | 0.6            | 0.1          |
